# Supplementary material for: Practically and Theoretically Efficient Garbage Collection for Multiversioning
Source: arXiv:2212.13557 source file (2023-01-08)
Supplement: Supplementary file 1 [file PPOPP-submission-supp.pdf]

## A Proofs for the Doubly-Linked List

**Invariant 2.** *Let  $C$  be a configuration and  $y$  be a node.*

1. *If  $y$  has been added to the list (and is not the sentinel), then  $y \rightarrow \text{left}$  is also a node that was added to the list and  $y \rightarrow \text{left} < y$ . For all  $w$ , if  $y \rightarrow \text{left} < w < y$  then  $w$  is marked.*
2. *If  $y \rightarrow \text{right}$  was non-null in a configuration at or before  $C$ , then in  $C$   $y \rightarrow \text{right}$  is a node that was added to the list and  $y \rightarrow \text{right} > y$ . For all  $w$ , if  $y < w < y \rightarrow \text{right}$  then  $w$  is marked.*
3. *For any call to  $\text{remove}(y)$  in progress, the local variables  $\text{left}$  and  $\text{right}$  are nodes that have been added to the list and  $\text{left} < y < \text{right}$ . Moreover, for all  $w$ , if  $\text{left} < w < \text{right}$  then  $w$  is marked.*
4. *The left pointer of the sentinel node is null.*

*Proof.* Initially, the only node is the sentinel node and its right pointer is null, and there is no pending call to remove, so the claim holds vacuously. We show that every step preserves each of the three claims of the invariant.

1. To prove that claim 1 is preserved, we must only consider steps that can add a node to the list or change the left pointer of a node.

When a node  $y$  is added to the list at line 18 of a call to  $\text{tryAppend}(x, y)$ ,  $y \rightarrow \text{left}$  has been set to  $x$  at line 17. By the preconditions, this is the unique call of the form  $\text{tryAppend}(*, y)$ , so a pointer to  $y$  has not previously been written into shared memory. So, no process could have updated  $y \rightarrow \text{left}$  and it is therefore still  $x$ . By the precondition of  $\text{tryAppend}$ ,  $x$  is a node that has previously been read from head, so it has been added to the list and  $x < y$ . Since the CAS on head changes it from  $x$  directly to  $y$ , there are no nodes  $w$  satisfying  $x < w < y$ .

The only instructions that update a left pointer are lines 17 and 33. As mentioned above, a node  $y$  has not been added to the list yet when line 17 of  $\text{tryAppend}(x, y)$  updates  $y \rightarrow \text{left}$ , so there is nothing more to prove. Suppose an execution of line 33 of a  $\text{remove}(x)$  sets  $y \rightarrow \text{left}$  to  $v$ . Then,  $v$  and  $y$  are the values of the remove's local variables  $\text{left}$  and  $\text{right}$ . By induction hypothesis 3,  $v$  has been added to the list and  $v < x < y$  and every node  $w$  satisfying  $v < w < y$  is marked. Thus, after the CAS, every node  $w$  satisfying  $y \rightarrow \text{left} < w < y$  is marked.

2. To prove that claim 2 is preserved, we must only consider steps that can change the right pointer of a node. The only instructions that set a right pointer to a non-null value are lines 16, 19 and 34.

First, consider line 19 of a  $\text{tryAppend}(x, y)$ , which sets  $x \rightarrow \text{right}$  to  $y$ . Since head was changed directly from  $x$  to  $y$  on line 18,  $y$  has been added to the list and  $x < y$ , and there are no nodes  $w$  satisfying  $x < w < y$ .

Next, consider an execution of line 34 of a  $\text{remove}(y)$  sets  $x \rightarrow \text{right}$  to  $z$ . Then,  $x$  and  $z$  are the values of

the local variables  $\text{left}$  and  $\text{right}$ . By the induction hypothesis,  $x < y < z$  and every node  $w$  satisfying  $x < w < z$  is marked. Thus, after the CAS, every node  $w$  satisfying  $x < w < x \rightarrow \text{right}$  is marked.

Finally, consider a CAS step  $s$  at line 16 of  $\text{tryAppend}(y, *)$  that changes  $x \rightarrow \text{right}$  from null to  $y$ . By the precondition of  $\text{tryAppend}$ ,  $y$  has been added to the list. The  $\text{tryAppend}$  read  $x$  from  $y \rightarrow \text{left}$  at line 14 before  $s$ . Since  $x$  is not null at line 16,  $y$  cannot be the sentinel node, by induction hypothesis 4. So  $x$  is a node that has been added to the list and  $x < y$  by induction hypothesis 1. We prove the remainder of the claim by showing that there is no  $w$  such that  $x < w < y$ . Since  $x \rightarrow \text{right}$  is null in the configuration before  $s$ , it follows from induction hypothesis 2 that

$$x \rightarrow \text{right} = \text{null at all times before } s. \quad (1)$$

Node  $x$  cannot be marked when  $s$  occurs: before a  $\text{remove}(x)$  could have marked  $x$ , a  $\text{tryAppend}(x, *)$  must have returned true (by the precondition for  $\text{remove}$ ), and that  $\text{tryAppend}$  would have set  $x \rightarrow \text{right}$  to a non-null value at line 19, contrary to (1).

To derive a contradiction, suppose there is some  $w$  such that  $x < w < y$ . Consider the minimal such  $w$  with respect to the total order  $<$ . (I.e.,  $w$  is the successor of  $x$  in the order  $<$ .) Since  $x \leftarrow y$  at line 14 before  $s$ ,  $w$  is marked, by induction hypothesis 1. This means that a  $\text{remove}(w)$  has been invoked before  $s$ . By the precondition of  $\text{remove}$ , a  $\text{tryAppend}(w, w')$  returned true before  $s$ , for some  $w'$ . Consider line 14 of that  $\text{tryAppend}$ . When it occurs,  $x$  is unmarked (since it is still unmarked at  $s$ ). By induction hypothesis 1,  $w \rightarrow \text{left} \geq x$  (since  $x$  is unmarked) and  $w \rightarrow \text{left} \leq x$  (since  $x$  is the predecessor of  $w$  in the order  $<$ ). Thus, line 14 reads  $x$  from  $w \rightarrow \text{left}$ . Line 16 of that  $\text{tryAppend}(w, w')$  (which also occurs before  $s$ ) will perform a  $\text{CAS}(x \rightarrow \text{right}, \text{null}, w)$ , violating (1). This contradiction proves that there is no  $w$  such that  $x < w < y$ .

3. We prove that claim 3 is preserved by all updates to the local variables  $\text{left}$  and  $\text{right}$  in a  $\text{remove}$  operation. By the precondition of  $\text{remove}(y)$ ,  $y$  is not the sentinel node. Moreover, a call to  $\text{tryAppend}(y, *)$  has returned true, so by the preconditions of  $\text{tryAppend}$ , we know that  $y$  has been added to the list before the  $\text{remove}$  begins. Moreover, the  $\text{tryAppend}$  executed line 19, after which  $y \rightarrow \text{right}$  is non-null. So, by induction hypothesis 2,  $y \rightarrow \text{right}$  points to a node that has been added to the list.

So, when the local variable  $\text{left}$  in the  $\text{remove}(y)$  operation is initialized on line 24 to the value read from  $y \rightarrow \text{left}$ , the claim follows from induction hypothesis 1. Similarly, when the local variable  $\text{right}$  is initialized

on line 25, the claim follows from induction hypothesis 2.

When the local variable `left` is advanced from  $x$  to  $x'$  at line 28 in a `remove(y)`, we have  $x' \leftarrow x$ . Since  $x$  is marked, so it is not the sentinel node, since the precondition to `remove` ensures that the sentinel node is never marked. By induction hypothesis 1,  $x' < x$  and each node  $w$  satisfying  $x' < w < x$  is marked. By induction hypothesis 3,  $x < y$  and each node  $w$  satisfying  $x < w < y$  is marked. Moreover, by the test on line 28,  $x$  is marked. The claim follows.

A symmetric argument shows that advancing the local variable `right` at line 29 also preserves the invariant.

4. Finally we show that claim 4 is preserved because no step can change the `left` pointer of the sentinel node. Line 17 of `tryAppend` changes the `left` field of a non-sentinel node, by the precondition to `tryAppend`. Consider a CAS step at line 33 of `remove(y)` that changes  $z \rightarrow \text{left}$ . By induction hypothesis 3,  $y < z$ , so  $z$  cannot be the sentinel node (which is the minimum element in the ordering  $<$ ).

□

**Lemma 3.** Suppose  $w < x < y < z$  and  $w \leftarrow y$  at some time during the execution. Then there is never a time when  $x \leftarrow z$ .

*Proof.* To derive a contradiction, suppose the claim is false.

Since there is a node  $x$  between  $w$  and  $y$  in the total order  $<$ , the head pointer takes the value  $x$  between the times it takes the values  $w$  and  $y$ . Thus,  $y$  is not added to the list by a `tryAppend(w, y)` operation, so the initial value of  $y \rightarrow \text{left}$  is not  $w$ . So, there is a CAS on line 33 of a `remove` operation that changes  $y \rightarrow \text{left}$  to  $w$ . This CAS was preceded by a test at line 32 that found  $y$  was not marked. At that time, the local variables `left` and `right` of the `remove` are equal to  $w$  and  $y$ . By Invariant 2.3,  $x$  is marked since  $w < x < y$ . Thus,  $x$  is marked before  $y$ .

An identical argument shows that a CAS at line 33 of a `remove` operation changes  $z \rightarrow \text{left}$  to  $x$  and at the execution of line 32 before that CAS,  $x$  is not marked and  $y$  is marked, so  $y$  is marked before  $x$ . This is a contradiction. □

**Lemma 4.** If line 33 does a CAS( $z \rightarrow \text{left}$ ,  $y$ ,  $w$ ), then  $w \leq y$ .

*Proof.* To derive a contradiction, suppose  $w > y$ . Consider the configuration  $C$  when  $y$  is read from  $z \rightarrow \text{left}$  on line 31 prior to the CAS. At  $C$ ,  $w$  and  $z$  are the values of the local variables `left` and `right` of the `remove`. By Invariant 2.3,  $w < z$ . In  $C$ , we have  $z \rightarrow \text{left} = y < w < z$ . By Invariant 2.1,  $w$  is marked in  $C$ . This contradicts the fact that  $w$  is unmarked when line 32 is executed after  $C$ . □

Recall that  $x \rightsquigarrow z$  if  $x$  can be reached from  $z$  by following `left` pointers. More formally,  $x \rightsquigarrow z$  if (a)  $x = z$  or (b) for some  $y$ ,  $y \leftarrow z$  and  $x \rightsquigarrow y$ .

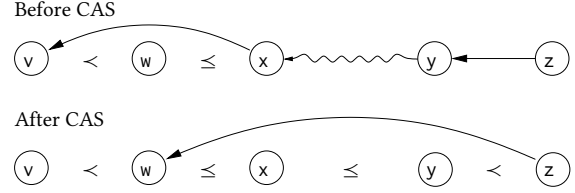

Figure 9. Proof of Lemma 5 and Lemma 16.

**Lemma 5.** If a CAS at line 33 changes  $z \rightarrow \text{left}$  from  $y$  to  $w$ , then  $w \rightsquigarrow y$  in the preceding configuration  $C$ .

*Proof.* Refer to Figure 9. Let  $x$  be the minimum node (with respect to  $<$ ) such that  $x \geq w$  and  $x \rightsquigarrow y$  in  $C$ . (This minimum is well-defined, since there exists a node  $x$  that satisfies both of these properties:  $y \geq w$  by Lemma 4 and  $y \rightsquigarrow y$  holds trivially.) Since  $x \rightsquigarrow y \leftarrow z$ , we have  $x < z$  by Lemma 2.1.

Let  $v$  be the value of  $x \rightarrow \text{left}$  in  $C$ . By Invariant 2.1,  $v < x$ . It must be the case that  $v < w$ ; otherwise we would have  $v \geq w$  and  $v \rightsquigarrow y$ , which would contradict the fact that  $x$  is the *minimum* node that satisfies these two properties.

To derive a contradiction, suppose  $w < x$ . Then we have  $v < w < x < z$ . We also have  $w \leftarrow z$  after the CAS and  $v \leftarrow x$  in  $C$ , which contradicts Lemma 3. Thus,  $w \geq x$ . By definition of  $x$ ,  $x \geq w$  and  $x \rightsquigarrow y$  in  $C$ . Thus,  $x = w$  and  $w \rightsquigarrow y$ . □

**Lemma 6.** When a node is removed from AL, it is marked.

*Proof.* A node can only be removed from the abstract list by a CAS step on a `left` pointer. Consider a CAS at line 33 that changes  $z \rightarrow \text{left}$  from  $y$  to  $w$ . By Invariant 2.1 and Lemma 5, only nodes  $x$  satisfying  $w < x < y$  can be removed from the abstract list by this CAS. Since  $w$  and  $y$  are the values of the local variables `left` and `right` in the `remove` operation that performs the CAS, Invariant 2.3 ensures that all such nodes  $x$  are marked when the CAS occurs. □

To ensure that we can linearize `remove` operations, we show that a `remove(x)` successfully removes  $x$  from the abstract list. The `remove` can only terminate when it performs a successful CAS on the `left` pointer of some node appended to the list after  $x$ . The following lemma shows that when that happens,  $x$  is no longer in the abstract list.

**Lemma 7.** When `remove(x)` terminates,  $x$  is not in AL.

*Proof.* Since the `remove(x)` terminates, it performs a successful CAS on a `left` pointer at line 33. Let  $w$  and  $z$  be the values of the `remove`'s local variables `left` and `right` when the CAS occurs. The CAS updates  $z \rightarrow \text{left}$  to  $w$ . By Invariant 2.3,  $w < x < z$ .

To derive a contradiction, suppose that  $x$  is still in the abstract list in the configuration  $C$  after this CAS.

Since  $x$  is in the abstract list and  $z \rightarrow \text{left} < x < z$ , there must be nodes  $v'$  and  $v$  in the abstract list such that  $x \rightsquigarrow$

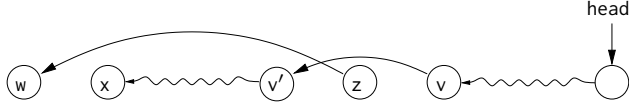

Figure 10. Proof of Lemma 7.

$v' \leftarrow v \rightsquigarrow \text{head}$  with  $v' < z < v$ . Refer to Figure 10. More formally, let  $v$  be the minimum node (with respect to the order  $<$ ) such that  $v \geq z$  and  $v \rightsquigarrow \text{head}$  in  $C$ . Let  $v' = v \rightarrow \text{left}$ . It follows from the definition of  $v$  that  $v' < z$ . If  $v$  were equal to  $z$ , then since  $x$  is in the abstract list,  $x$  would have to be reachable by following left pointers from  $w$ , which would violate 2.1, since  $w < x$ . Thus,  $v > z$ .

So, we have  $w < x \leq v' < z < v$  and  $w \leftarrow z$  and  $v' \leftarrow v$ , which violates Lemma 3.  $\square$

We now specify the linearization points of update operations so that we maintain the invariant that, for all configurations  $C$ , the abstract list  $L_C$  in that configuration is exactly the list that would be obtained by performing the operations linearized before  $C$  in their linearization ordering. We linearize a successful `tryAppend` operation (i.e., one that returns `true`) when it updates the head pointer at line 18. We linearize a `remove(x)` when a CAS at line 33 removes  $x$  from the abstract list. This step may be performed by the `remove` itself or by another `remove` operation. By Lemma 5,  $n$  will remain out of the abstract list forever once it is removed. By Lemma 6, only marked nodes are removed from the abstract list when a left pointer is updated. By Lemma 7, there is a well-defined linearization point for each `remove` operation that terminates, and it is before the `remove` terminates. By Lemma 6, it is also after the `remove` operation performs line 23, so the linearization point is during the execution interval of the `remove`. Thus, the linearization is consistent with the abstract list.

A CAS of a left pointer may remove several nodes from the abstract list, and therefore be used as the linearization point of several `remove` operations. When linearizing such a batch of `remove` operations, we order them in decreasing order by  $<$ . In other words, we remove the batch of nodes from right to left. Thus, when a CAS on a left pointer splices several nodes out of the abstract list, we can think of the abstract list as undergoing a sequence of changes by performing those `remove` operations one by one. This will be important, because it is sometimes necessary to linearize searches in the *middle* of such a batch of `remove` operations.

We now describe how to linearize search operations. It is a common technique to argue that each node visited by a search was in the data structure at some time during the search (e.g., [14, 37]). Such proofs often rely on the fact that once a node is removed from the data structure, its pointers can no longer be changed. This does not hold for our data structure, but we can still establish the required property

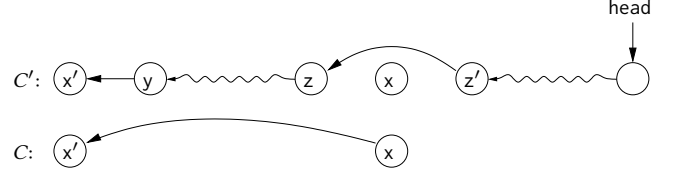

Figure 11. Proof of Lemma 8.

using Lemmas 3 and 5. (An alternative approach would be to use the forepassed condition defined in [17].)

**Lemma 8.** *Let  $C$  be a configuration and  $x$  be the local variable of a pending `search(k)` in  $C$ . There was a time between the invocation of the search and  $C$  when  $x$  was in AL and either  $x$  was the first node in AL or its predecessor in AL had a key greater than  $k$ .*

*Proof.* Consider any `search(k)` operation in the execution. We prove the claim holds for every configuration  $C$  during the search by induction on the number of steps the search has performed.

For the base case, consider the configuration  $C$  after the search is invoked and executes line 9,  $x$  is initialized to head, so it is the first node in the abstract list in  $C$ .

For the induction step, we must just verify that steps that modify the local variable  $x$  preserve the claim. Consider an execution of line 11 that advances the search from node  $x$  to  $x'$ , and let  $C$  be the configuration after that step. Then, in  $C$ ,  $x' \leftarrow x$ . By the test at line 10,  $x \rightarrow \text{key} > k$ .

First, consider the case where  $x$  is in  $L_C$ . Since  $x' \leftarrow x$  in  $C$ ,  $x'$  is also in  $L_C$  and its predecessor  $x$  in  $L_C$  has a key greater than  $k$ . Thus, the claim is satisfied at  $C$ .

So, for the remainder of the proof, assume  $x$  is not in  $L_C$ . By the induction hypothesis, there was an earlier time during the search when  $x$  was in the abstract list. So there was a CAS step  $s$  during the search that removed  $x$  from the abstract list.

Lemma 5 implies that if  $x' \rightsquigarrow x$  after some CAS on a left pointer, then  $x' \rightsquigarrow x$  before that CAS too. Since  $x' \rightsquigarrow x$  in  $C$ , it follows that  $x' \rightsquigarrow x$  holds in all configurations between the addition of  $x$  to the abstract list and  $C$ . In particular, this means that  $x' \rightsquigarrow x$  in the configuration before  $s$ . So  $x'$  is in the abstract list in that configuration. We consider the two possible cases.

- Suppose  $s$  removes both  $x$  and  $x'$  from the abstract list. Then  $s$  removes some sequence of nodes from the abstract list by updating the left pointer of some node  $z$ . Since we linearize a batch of `remove` operations from right to left,  $z$  is the predecessor of  $x'$  in the abstract list just before the linearization of `remove(x')`. It follows from Lemma 5 that  $x \rightsquigarrow z$  in the configuration before  $s$ . By the precondition that the list is always sorted, we have  $z \rightarrow \text{key} \geq x \rightarrow \text{key} > k$ . Thus, the



claim is satisfied just before the linearization point of the  $\text{remove}(x')$ .

- Suppose  $x'$  is still in the abstract list in the configuration  $C'$  following  $s$ . If  $x'$  is the first element of  $L_{C'}$ , then the claim holds.

Otherwise, there is some  $y$  such that in  $C'$ ,  $x' \leftarrow y \leftarrow \text{head}$ . To derive a contradiction, suppose  $y < x$ . Then there must be nodes  $z$  and  $z'$  such that  $y \leq z < x < z'$  and  $y \leftarrow z \leftarrow z' \leftarrow \text{head}$  in  $C'$ . (See Figure 11: at some point in the path from head to  $y$ , there must be consecutive nodes  $z \leftarrow z'$  such that  $z < x < z'$  since  $x$  is not in the abstract list.) So we have  $x' < x < x < z'$  and  $z \leftarrow z'$  in  $C'$  and  $x' \leftarrow x$  in  $C$ . This violates Lemma 3. Hence,  $y \geq x$ . We cannot have  $y = x$ , since  $y$  is in  $L_{C'}$  and  $x$  is not. So,  $y > x$ . By the precondition that nodes are appended with non-decreasing keys, this means that  $y \rightarrow \text{key} \geq x \rightarrow \text{key} > k$ . So,  $x'$  is in  $L_{C'}$  and its predecessor  $y$  has a key greater than  $k$ , as required.

□

Suppose a  $\text{search}(k)$  returns the value of a node  $x$ . By the exit condition on line 10,  $v_x \rightarrow \text{key} \leq k$ . Lemma 8 says there is a time during the search when  $x$  is in the abstract list and its predecessor in the list has a key greater than  $k$ . Thus, at that time,  $x$  is the first node in the abstract list whose key is less than or equal to  $k$ . We choose that time as the linearization point of the search.

## B Correctness of the Singly-Linked List

We assume that the following preconditions are satisfied.

1. If  $\text{tryAppend}(x, y)$  is invoked, then  $x$  has been read from head, and no other  $\text{tryAppend}(*, y)$  has been invoked.
2. If a node  $x$  is appended to the list before  $y$ ,  $x.\text{ts} \leq y.\text{ts}$ .
3. While a  $\text{search}(t)$  is in progress,  $t$  appears in  $\text{Announce}$ .
4. At all times after a  $\text{compact}(A, t, *)$  is invoked and for all  $i$ , either  $\text{Announce}[i] \in A$  or  $\text{Announce}[i] \geq t$ .

These conditions are satisfied naturally in MVGC applications. Since  $\text{compact}$  takes its parameters from an  $\text{AnnScan}$  object  $(A, t)$ ,  $\text{scanAnnounce}$  ensures that  $t$  was copied from shared memory before  $A$ . Since the global timestamp is non-decreasing, any value stored in  $\text{Announce}[i]$  after that entry was copied into  $A$  will be greater than  $t$ . (We assume  $\text{rtxs}$  announcing a timestamp copy the global timestamp into  $\text{Announce}$  atomically, as described in [47]. An optimization that avoids this is described in Appendix B.2.)

As in Section 4.1, we say a node is appended to the list when a pointer to the node is stored in head. We consider the sentinel node to be appended to the list when the list is created. We also use the notation  $x \leftarrow y$  and  $x < y$  as in Section 4.1. We first prove some simple facts about the algorithm.

### Invariant 9.

1. If  $y$  has been appended to the list and is not the sentinel node and  $w \leftarrow y$  then  $w$  is a node that has been appended to the list and  $w < y$ .
2. If a CAS at line 28 changes  $y \rightarrow \text{left}$  from  $x$  to  $w$ , then  $w < x$ .
3. A compact never sets  $\text{cur}$ ,  $\text{next}$  or  $\text{newNext}$  to null.

*Proof.* We show that each step preserves the invariant. Assume the invariant holds prior to the step. We need only consider steps that append a node, successfully CAS a left pointer and update the local variables  $\text{cur}$ ,  $\text{next}$  and  $\text{newNext}$ .

First, consider a step that appends a node  $y$  to the list (line 34). If  $w \leftarrow y$  when  $y$  is appended to the list by a CAS at line 34, then head is changed from  $w$  directly to  $y$ . Thus,  $w$  is a node that was appended to the list before  $y$ .

The only step that changes a left pointer after it is initialized is a successful CAS at line 28. Suppose this step changes  $y \rightarrow \text{left}$  from  $x$  to  $w$ . Then,  $x$  and  $w$  are the values of local variables  $\text{next}$  and  $\text{newNext}$  when the CAS occurs. Prior to the CAS,  $w$  has been reached from  $y$  by following left pointers, first at line 16 and then at lines 25–27. Moreover, before advancing from one node to the next by reading a left pointer (at line 16, 25 or 27), the algorithm first checks (at line 15, 22 or 26, respectively) that the former node is not the sentinel, either explicitly, or by checking that the node's  $\text{ts}$  field is greater than  $A[i]$ . Since the invariant holds before the CAS,  $w$  has been appended and  $w < x < y$ .

As mentioned in the previous paragraph, when we set  $\text{next}$  at line 16 or set  $\text{newNext}$  at lines 25 or 27 by reading the left field of a node, we first check that that node is not the sentinel. Since the invariant holds before reading this left field, the value we store in  $\text{next}$  or  $\text{newNext}$  is non-null. Similarly, if  $\text{next}$  is updated at line 29, the test at line 15 guarantees that  $\text{cur}$  is not the sentinel, so its left pointer is non-null.

We check that all steps that set the  $\text{cur}$  variable give it a non-null value. The  $\text{cur}$  variable is set to the value read from head at line 14, and head is never null. Lines 19 and 23 copy the value  $\text{next}$  into  $\text{cur}$ , and this value is non-null, by the induction hypothesis. Line 31 sets  $\text{cur}$  to the value read from the left field of a node that is known not to be the sentinel (by the test at line 15), so its left field is non-null by the induction hypothesis. □

It follows from Invariant 9 that all pointers dereferenced in compact are non-null.

The following technical lemma shows that compact updates  $i$  appropriately to carry out the test of whether node  $\text{next}$  is needed.

**Lemma 10.** *If the test on line 22 fails, then either  $i$  is the index of the last entry of  $A$  or  $\text{cur} \rightarrow \text{ts} \leq A[i+1]$ .*

*Proof.* Let  $C$  be the configuration after the test on line 22 fails. Consider the configuration  $C_i$  after the last time the local variable  $i$  was updated prior to  $C$ . If this was when  $i$  was

initialized at line 13, then  $i$  is the index of the last element of  $A$ , which makes the claim true. Otherwise,  $i$  was updated at line 21. Then,  $A[i+1] \geq \text{cur} \rightarrow \text{ts}$  held at  $C_i$ . Between  $C_i$  and  $C$ , we argue that changes to  $\text{cur}$  can only cause  $\text{cur} \rightarrow \text{ts}$  to decrease. If  $\text{cur}$  is updated at line 19 or 23 it is changed to the value read from the `left` pointer of the previous  $\text{cur}$  node at line 16. Similarly, line 31 updates  $\text{cur}$  to the value read from the `left` pointer of the previous  $\text{cur}$  node. By Lemma 9 and precondition 2, updating  $\text{cur}$  between  $C_i$  and  $C$  by traversing `left` pointers cannot cause  $\text{cur} \rightarrow \text{ts}$  to increase. Thus, at  $C$ , we still have  $\text{cur} \rightarrow \text{ts} \leq A[i+1]$ .  $\square$

We say that  $(A, t)$  is *written before*  $(A', t')$  if an `AnnScan` object  $(A, t)$  is stored in `GlobalAnnScan` before  $(A', t')$ . The following lemma is proved using the fact that creating the earlier copy completes before creating the later copy begins, because of the way we use CAS to update `GlobalAnnScan`. This, in turn, guarantees that once a node becomes unneeded, it is never needed by a later `AnnScan` pair.

**Lemma 11.** *Suppose  $(A_1, t_1)$  is written before  $(A_2, t_2)$ . For any node  $x$ , if  $x$  is needed  $(A_2, t_2)$  then  $x$  is needed  $(A_1, t_1)$ .*

*Proof.* Since every CAS on `GlobalAnnScan` tries to install a newly created object, there is no ABA problem on `GlobalAnnScan`. Thus, `GlobalAnnScan` is not updated between the time it is read on line 6 and the time a successful CAS is applied to it on line 9. Thus,  $(A_1, t_1)$  is stored in `GlobalAnnScan` before the process that stores  $(A_2, t_2)$  begins reading the values  $(A_2, t_2)$  from the `Announce` array and the global timestamp. Thus,  $t_1 \leq t_2$ . Moreover, if some value  $t < t_1$  appears in  $A_2$ , then it must also appear in  $A_1$  since we assume values written into the `Announce` array are atomically copied from the global timestamp.

Assume  $x$  is needed  $(A_2, t_2)$ . We consider several cases.

If  $x.\text{ts} > t_1$ , then  $x$  is also needed  $(A_1, t_1)$ , by definition.

If  $x.\text{ts} \leq t_1$  and  $x$  is the last appended node with timestamp at most  $t_2$ , then it is also the last appended node with timestamp at most  $t_1$  since  $t_1 \leq t_2$ . Thus,  $x$  is needed  $(A_1, t_1)$ .

Otherwise,  $x.\text{ts} \leq t_1$  and  $x$  is the last appended node with timestamp at most  $A_2[i]$  for some  $i$ . If  $A_2[i] \geq t_1$ , then  $x$  is also the last appended node with timestamp at most  $t_1$ , and is therefore needed  $(A_1, t_1)$ . If  $A_2[i] < t_1$  then the value  $A_2[i]$  must also appear in  $A_1$ . So, again  $x$  is needed  $(A_1, t_1)$ .  $\square$

The following key lemma describes how a `compact`  $(A, t, *)$  works: it traverses nodes that are needed  $(A, t)$  and splices out those nodes that are not needed  $(A, t)$ . The proof is necessarily quite technical because, even though the set of needed nodes can only be reduced when `GlobalAnnScan` is updated, there many `compact` routines simultaneously traversing a version list, whose arguments are  $(A, t)$  pairs read from `GlobalAnnScan` at different times—some out of date and some more current.

**Lemma 12.** *If an invocation of `compact`  $(A, t, h)$  sets its local variable `cur` to a node  $x \neq h$ , then  $x$  is needed  $(A, t)$ . If*

*an invocation of `compact`  $(A, t, h)$  performs a successful CAS that stores  $v$  in `x`  $\rightarrow$  `left`, then  $x$  is needed  $(A, t)$  (unless  $x = h$ ) and  $v$  is needed  $(A, t)$  and for all  $w$  satisfying  $v < w < x$ ,  $w$  is not needed  $(A, t)$ .*

*Proof.* We prove the lemma by induction on steps: we assume the lemma is true in a prefix of an execution and show that it remains true when an additional step  $s$  is appended to the prefix. We first prove a couple of technical claims that will be used several times in the induction step.

**Claim 12.1.** *If  $x \leftarrow z$  at some time before  $s$  and either  $x.\text{ts} \leq A[j] < z.\text{ts}$  for some  $j$  or  $z.\text{ts} > t$ , then  $x$  is needed  $(A, t)$ .*

*Proof of Claim.* We consider several cases.

1. If  $x.\text{ts} > t$ , then  $x$  is needed  $(A, t)$  by definition.
2. If  $x$  is the last appended node whose timestamp is at most  $t$ , then  $x$  is needed  $(A, t)$  by definition.
3. Suppose  $x.\text{ts} \leq t < z.\text{ts}$  but  $x$  is not the last node whose timestamp is at most  $t$ . Let  $y$  be the last appended node whose timestamp is at most  $t$ . By definition,  $y$  is needed  $(A, t)$ . Since  $z.\text{ts} > t$ , we have  $x < y < z$  by precondition 2. By the hypothesis of the claim, some invocation `compact`  $(A', t')$  set  $z \rightarrow \text{left}$  to  $x$  before  $s$ . By the induction hypothesis,  $x$  is needed  $(A', t')$  but  $y$  is not needed  $(A', t')$ . Since  $y$  is needed  $(A, t)$  but not needed  $(A', t')$ ,  $(A, t)$  is written before  $(A', t')$ , by Lemma 11. Since  $x$  is needed  $(A', t')$ ,  $x$  is also needed  $(A, t)$ , again by Lemma 11.
4. If  $x$  is the last appended node whose timestamp is at most  $A[j]$  (for some  $j$ ), then  $x$  is needed  $(A, t)$ , by definition.
5. Otherwise,  $x.\text{ts} \leq A[j] < z.\text{ts}$  for some  $j$ , but  $x$  is not the last appended node with timestamp at most  $A[j]$ . This case is very similar to Case 3. Let  $y$  be the last appended node whose timestamp is at most  $A[j]$ . By definition,  $y$  is needed  $(A, t)$ . Since  $z.\text{ts} > A[j]$ , we have  $x < y < z$  by precondition 2. By the hypothesis of the claim, some invocation `compact`  $(A', t')$  set  $z \rightarrow \text{left}$  to  $x$  before  $s$ . By the induction hypothesis,  $x$  is needed  $(A', t')$  but  $y$  is not needed  $(A', t')$ . Since  $y$  is needed  $(A, t)$  but not needed  $(A', t')$ ,  $(A, t)$  is written before  $(A', t')$ , by Lemma 11. Since  $x$  is needed  $(A', t')$ ,  $x$  is also needed  $(A, t)$ , again by Lemma 11.

$\square$

**Claim 12.2.** *If  $s$  is an execution of line 28 or 31, let  $v$  and  $x$  be the nodes stored in `newNext` and `cur`, respectively, in the configuration before  $s$ . Then  $v < x$  and  $v$  is needed  $(A, t)$  and for all  $w$  satisfying  $v < w < x$ ,  $w$  is not needed  $(A, t)$ .*

*Proof of Claim.* The node  $v$  was reached from  $x$  by following `left` pointers, at line 16 and then at lines 25–27. By Invariant 9,  $v < x$ . Let  $x = w_1, w_2, \dots, w_k = v$  be the sequence of nodes traversed to get from  $x$  to  $v$ . By the tests on lines 22 and 26,

$w_k.ts \leq A[i] < w_{k-1}.ts$ . Since  $w_k$  was read from  $w_{k-1}$  before  $s$ , Claim 12.1 implies that  $v = w_k$  is *needed*( $A, t$ ).

It remains to show that all nodes  $w$  satisfying  $v < w < x$  are not *needed*( $A, t$ ). Since the test at line 18 failed,  $x.ts \leq t$ . So a node  $w < x$  cannot be the last appended node with timestamp at most  $t$ , nor can  $w$  have a timestamp greater than  $t$ . To complete the proof that  $w$  is not *needed*( $A, t$ ), we must show that it is not the last appended node with timestamp at most  $A[j]$  for any  $j$ . We do this in two parts, first considering  $j > i$  and then  $j \leq i$ . (Recall that  $A[0] = -1$ .)

Since  $x$  is the value of  $cur$  when the test at line 22 fails, it follows from Lemma 10 that either  $i$  is the index of the last element of  $A$  or  $x \rightarrow ts \leq A[i + 1]$ . Thus, any node  $w < x$  cannot be the last appended node whose timestamp is at most  $A[j]$  for any  $j > i$ , since then  $i$  would not be the last index and so  $x.ts \leq A[i + 1] \leq A[j]$ .

To derive a contradiction, suppose that there is some  $w$  such that  $v < w < x$  and  $w$  is *needed*( $A, t$ ). Since we have already eliminated all other possibilities, this means that for some  $j \leq i$ ,  $w$  is the last appended node whose timestamp is at most  $A[j]$ . Since  $w.ts \leq A[j] \leq A[i] < w_{k-1}.ts$ , we must have  $v = w_k < w < w_{k-1}$ . (In particular, this means that  $w_{k-1}$  cannot be *needed*( $A, t$ ).) Since  $w_k$  was read before  $s$  from  $w_{k-1} \rightarrow left$ , the induction hypothesis implies that some  $compact(A', t')$  did a CAS that set  $w_{k-1} \rightarrow left$  to  $w_k$  and  $w_{k-1}$  is *needed*( $A', t'$ ) but  $w$  is not *needed*( $A', t'$ ). Since  $w_{k-1}$  is *needed*( $A', t'$ ) but not *needed*( $A, t$ ), Lemma 11 implies that the  $AnnScan$  object  $(A', t')$  is written before  $(A, t)$ . Since  $w$  is not *needed*( $A', t'$ ), it follows from Lemma 11 that  $w$  is not *needed*( $A, t$ ). This contradiction completes the proof of the claim.  $\square$

Now we are ready to prove that step  $s$  preserves the truth of the lemma. We need only consider steps  $s$  that update the  $cur$  variable of a  $compact$  routine or perform a successful CAS at line 28.

Now, suppose  $s$  executes line 19 to change the  $cur$  pointer from node  $z$  to  $x$ . Then  $x$  was read from  $x \rightarrow left$  at line 16. By the test at line 18,  $z.ts > t$ . So, by Claim 12.1,  $x$  is *needed*( $A, t$ ).

Now, suppose  $s$  executes line 23 to change the  $cur$  pointer from node  $z$  to  $x$ . Then,  $x$  was read from  $x \rightarrow left$  at line 16. Since the while loop at line 21 terminated, we have  $z.ts > A[i]$ . By the test at line 22, we have  $x \leq A[i]$ . So, by Claim 12.1,  $x$  is *needed*( $A, t$ ).

Now, suppose  $s$  performs a successful CAS at line 28 that changes  $x \rightarrow left$  to  $v$ . Then  $x$  and  $v$  are the values of the local variables  $cur$  and  $newNext$ , respectively, when the CAS occurs. Since  $x$  is stored in  $cur$ ,  $x$  is *needed*( $A, t$ ), by the induction hypothesis. Claim 12.2 says that  $v$  is *needed*( $A, t$ ) and any node  $w$  satisfying  $v < w < x$  is not *needed*( $A, t$ ).

Finally, suppose  $s$  executes line 31 to change the  $cur$  pointer from node  $z$  to  $w$ . Let  $y$  be the node stored in  $newNext$ . By Claim 12.2,  $y < z$  and  $y$  is *needed*( $A, t$ ). We argue that,

prior to  $s$ , a node  $x \leq y$  was stored in  $z \rightarrow left$  by considering two cases. If the loop at lines 28–30 terminated because the CAS at line 28 succeeded, then that CAS stored  $y$  in  $z \rightarrow left$ . Otherwise, the test at line 30 was true, so the node  $x$  read from  $z \rightarrow left$  on line 29 satisfied  $x.ts \leq y.ts$ . Since the test at line 18 failed,  $z.ts \leq t$ . Since  $y < z$ ,  $y.ts \leq z.ts \leq t$  by precondition 2. Since  $y$  is *needed*( $A, t$ ), it must be the last appended node with its timestamp. Therefore,  $x.ts \leq y.ts$  implies that  $x \leq y$ . Thus, in either case, a node  $x \leq y$  was stored in  $z \rightarrow left$  before  $s$ . By Lemma 9, the node  $w$  that  $s$  reads in  $z \rightarrow left$  satisfies  $w \leq x$ . We show that  $w$  is *needed*( $A, t$ ) by considering two cases. If  $w = y$ , we already know that  $y$  is *needed*( $A, t$ ). If  $w \neq y$ , we have  $w \leq x \leq y < z$ . Assume the CAS that stored  $w$  in  $x \rightarrow left$  was performed by a  $compact(A', t')$ . By the induction hypothesis,  $y$  is not *needed*( $A', t'$ ) since  $w < y < z$  and a CAS in  $compact(A', t')$  stored  $w$  in  $z \rightarrow left$ . Since  $y$  is *needed*( $A, t$ ), Lemma 11 implies that  $(A, t)$  was written before  $(A', t')$ . Since  $w$  is *needed*( $A', t'$ ), it follows from Lemma 11 that  $w$  is *needed*( $A, t$ ).  $\square$

We linearize successful  $tryAppend$  operations when they CAS the head pointer of the list. We linearize a search operation when it reads the head at line 36. The following theorem guarantees that every search operation returns the correct response.

**Theorem 13.** *If a  $search(k)$  operation returns the value from the last node appended to the list before the linearization point of the search whose timestamp is at most  $k$ .*

*Proof.* The search returns the value from the node stored in the local variable  $x$ .

If  $x$  is the value read from head at line 36, then  $x$  is the last node appended to the list before the linearization point of the search, and its timestamp is at most  $t$  since the test at line 37 failed.

Otherwise, there is a configuration  $C$  during the search just before  $x$  is read from the  $left$  pointer of some node  $z$  at line 38. By the test at line 37, we know that  $x \rightarrow ts \leq t < z \rightarrow ts$ . To derive a contradiction, suppose  $x$  is not the last appended node whose timestamp is at most  $k$ . Let  $y$  be the last appended node whose timestamp is at most  $k$ . Then,  $x < y < z$ .

By Lemma 12, there is an invocation of  $compact(A, t)$  before  $C$  such that  $y$  is not *needed*( $A, t$ ). We consider two cases.

If  $k \in A$ , then  $y$  is not the last appended node whose timestamp is at most  $k$ , since  $y$  is not *needed*( $A, t$ ). This is the desired contradiction.

Otherwise,  $k \notin A$ . At  $C$ ,  $k$  is in the  $Announce$  array, by precondition 3. By precondition 4, this means that  $k \geq t$ . Since  $y$  is not *needed*( $A, t$ ),  $y \rightarrow ts \leq t$ , and there is a node appended after  $y$  whose timestamp is also at most  $t$ . Since  $k \geq t$ , there is another node appended after  $y$  whose timestamp is at most  $k$ . Again, this is a contradiction.  $\square$



## B.1 Analysis

We now consider progress properties. We use Invariant 9 to prove wait-freedom and that search does not fall off the end of the list.

**Lemma 14.** *The compact and search routines are wait-free. A search never sets its local variable  $x$  to null.*

*Proof.* We first show that compact is wait-free. Each iteration of the outer loop updates  $\text{cur} \rightarrow \text{left}$  at line 19, 23 or 31 to a value read from  $\text{cur} \rightarrow \text{left}$  at line 16 or 31. Consider the sequence of values  $x_1, x_2, \dots$  assigned to the  $\text{cur}$  variable of the compact routine. By Invariant 9, all the values are non-null and we have  $x_1 > x_2 > \dots$ . Since there are finitely many nodes that precede  $x_1$  in the order  $<$ , the loop will terminate.

We must also check that the inner loops terminate. Due to the test at line 15,  $\text{cur}$  is not the sentinel node when the loop at line 21 is executed. Thus,  $\text{cur} \rightarrow \text{ts} \geq 0$ , so when the index  $i$  reaches 0,  $A[0] = -1 < \text{cur} \rightarrow \text{ts}$  and the loop terminates. (This argument also ensures that we never use an out-of-bounds index for  $A$ .)

Each iteration of the loop at lines 26–27 sets  $\text{newNext}$  to an earlier node in the order  $<$ , by Invariant 9. So, it must terminate.

Each time the test at line 28 fails, some other operation has performed a successful CAS on  $\text{cur} \rightarrow \text{left}$ . By Invariant 9, each such CAS changes  $\text{cur} \rightarrow \text{left}$  to an earlier node in the order  $<$ , so it must eventually terminate.

We now show that search is wait-free and does not set  $x$  to null. Line 36 initializes  $x$  to the node read from  $\text{head}$ , which has been appended (by definition). If line 38 changes  $x$ , then the node previously stored in  $x$  was not the sentinel, since its timestamp was greater than  $k \geq 0$ . Thus, the value read from its left pointer is non-null, by Lemma 9.

If the sequences of nodes visited by the search is  $x_1, x_2, \dots$ , then by Lemma 9, we have  $x_1 > x_2 > \dots$ . Since there are only finitely many nodes that precede  $x_1$  in the order  $<$ , the loop must terminate.  $\square$

For PDL, we proved Lemmas 3 and 5 to show that CAS steps on left pointers can only remove nodes; they cannot cause a remove node to return to the list. We now prove analogous results for SSL.

**Lemma 15.** *Suppose  $w < x < y < z$  and  $w \leftarrow y$  at some time during the execution. Then there is never a time when  $x \leftarrow z$ .*

*Proof.* To derive a contradiction, suppose the claim is false.

Since there is a node  $x$  between  $w$  and  $y$  in the total order  $<$ , the head pointer takes the value  $x$  between the times it takes the values  $w$  and  $y$ . Thus,  $y$  is not added to the list by a  $\text{tryAppend}(w, y)$  operation, so the initial value of  $y \rightarrow \text{left}$  is not  $w$ . So, there is a CAS on line 28 of a compact( $A, t, h$ ) operation that changes  $y \rightarrow \text{left}$  to  $w$ . Similarly, there is a

CAS of a compact( $A, t, h$ ) operation that changes  $z \rightarrow \text{left}$  to  $x$ . By Lemma 12,  $x$  is *needed*( $A', t'$ ) but not *needed*( $A, t$ ). By Lemma 11, ( $A', t'$ ) is written before ( $A, t$ ). Since the arguments of compact are obtained by taking a snapshot of GlobalAnnScan and head, this means that  $h'$  was stored in head before  $h$ , so  $h' \leq h$ . Thus,  $w < x \leq h' \leq h$ , so  $w \neq h$ . By Lemma 12,  $w$  is *needed*( $A, t$ ) but not *needed*( $A', t'$ ). This contradicts Lemma 11.  $\square$

**Lemma 16.** *If a CAS at line 28 changes  $z \rightarrow \text{left}$  from  $y$  to  $w$ , we have  $w \rightsquigarrow y$  in the preceding configuration  $C$ .*

*Proof.* Refer to Figure 9. Let  $x$  be the minimum node (with respect to  $<$ ) such that  $x \geq w$  and  $x \rightsquigarrow y$  in  $C$ . (This minimum is well-defined, since there exists a node  $x$  that satisfies both of these properties:  $y \geq w$  by Lemma 4 and  $y \rightsquigarrow y$  holds trivially.) Since  $x \rightsquigarrow y \leftarrow z$ , we have  $x < z$  by Lemma 9.

Let  $v$  be the value of  $x \rightarrow \text{left}$  in  $C$ . By Lemma 9,  $v < x$ . It must be the case that  $v < w$ ; otherwise we would have  $v \geq w$  and  $v \rightsquigarrow y$ , which would contradict the fact that  $x$  is the *minimum* node that satisfies these two properties.

To derive a contradiction, suppose  $w < x$ . Then we have  $v < w < x < z$ . We also have  $w \leftarrow z$  after the CAS and  $v \leftarrow x$  in  $C$ , which contradicts Lemma 15. Thus,  $w \geq x$ . By definition of  $x$ ,  $x \geq w$  and  $x \rightsquigarrow y$  in  $C$ . Thus,  $x = w$  and  $w \rightsquigarrow y$ .  $\square$

Lemma 16 allows us to prove that the compact routine permanently removes unneeded nodes.

**Proposition 17.** *Suppose a compact( $A, t, h$ ) routine on a version list has terminated prior to some configuration  $C$ . Then all nodes  $x$  satisfying  $\text{sentinel} < x < h$  that are reachable from the head of the version list in  $C$  are *needed*( $A, t$ ).*

*Proof.* To derive a contradiction, assume that some node  $x$  is reachable from head in  $C$  and  $x$  is not *needed*( $A, t$ ). Consider the sequence of values  $h = y_1, y_2, \dots, y_\ell = \text{sentinel}$  that are assigned to the local variable  $\text{cur}$  during the compact( $A, t, h$ ) routine. Since each is read from the left pointer of the previous one,  $y_\ell < y_{\ell-1} < \dots < y_1$ . Since  $x$  is not *needed*( $A, t$ ), Lemma 12 implies that  $x$  does not appear in this sequence. So, for some  $j$ ,  $y_{j+1} < x < y_j$ .

Now, let  $\text{head} = z_1, z_2, \dots, z_k = x$  be the path from head to  $x$  by following left pointers. Consider the maximum  $i$  such that  $z_i \geq y_j$ . (Such an  $i$  exists, since  $z_1 = \text{head} \geq h = y_1 \geq y_j$ .) So, we have  $y_{j+1} < x = z_k < z_{k-1} < \dots < z_{i+1} < y_j \leq z_i$ . Now,  $y_{j+1} \leftarrow y_j$  at some time during the compact (before  $C$ ). If  $y_j$  were equal to  $z_i$ , then in  $C$ ,  $z_i \rightarrow \text{left} = y_j \rightarrow \text{left} \leq y_{j+1}$  by Invariant 9, and this would contradict the fact that  $z_i \rightarrow \text{left} = z_{i+1} > y_{j+1}$ . So, we have  $y_{j+1} < z_{i+1} < y_j < z_i$ . However,  $y_{j+1} \leftarrow y_j$  at some time before  $C$  and  $z_{i+1} \leftarrow z_i$  in  $C$ . This contradicts Lemma 15.  $\square$

The head of a version list represents the current version, so it is not obsolete. Thus, when a node is added to the

range tracker data structure, it is no longer the head of its list. Once a process receives a node  $x$  returned by the range tracker, it gets up-to-date copies  $A$ ,  $t$  and  $h$  of the announcements, global timestamp and the list's head and invoke  $\text{compact}(A, t, h)$ . Since  $x$  was already returned by the range tracker,  $x$  will not be  $\text{needed}(A, t)$  and  $x < h$ . Proposition 17 ensures that  $x$  is permanently removed from its version list before the  $\text{compact}$  terminates. Thus, aside from the lists where  $\text{compact}$  routines are still pending, all nodes that have been returned by the range tracker are no longer reachable from the head of the list.

## B.2 Reserving Timestamps

Both BBF+ and our singly-linked list compaction algorithm from Section 5 use atomic copy (a primitive which allows us to atomically read from one memory location and write to another) to announce timestamps in a wait-free manner. Instead, in our experiments, we use a lighter-weight lock-free scheme for announcing timestamps which consist of (A1) reading the current timestamp, (A2) announcing it, and (A3) checking if the current timestamp is still equal to the announced value and, if not, going back to step A1. This means that a process scanning the announcement array might see a very old timestamp get announced, which breaks the monotonicity property required for the correctness of our singly-linked list. We fix this by having all processes work on updating a global scan of the announcement array as described in Section 5. When reading the announcement array, we ignore any timestamp that (1) is smaller than the timestamp at which the current global scan was taken and (2) does not appear in the current global scan. This is safe because any announced timestamp satisfying these two conditions will fail the check in step A3, and not be used. This change to how we scan announcement arrays ensures that the global scan satisfies the monotonicity property required by our singly-linked list. This announcement scanning technique is also used in our implementation of STEAM+LF, BBF+, and SL-RT.

## C Additional Experiments

Figures 12–16 showcase the same workloads as Figures 4–8, but with keys drawn from uniform rather than zipfian distribution.



Legend for all figures: SL-RT DL-RT BBF+ Steam+LF EBR

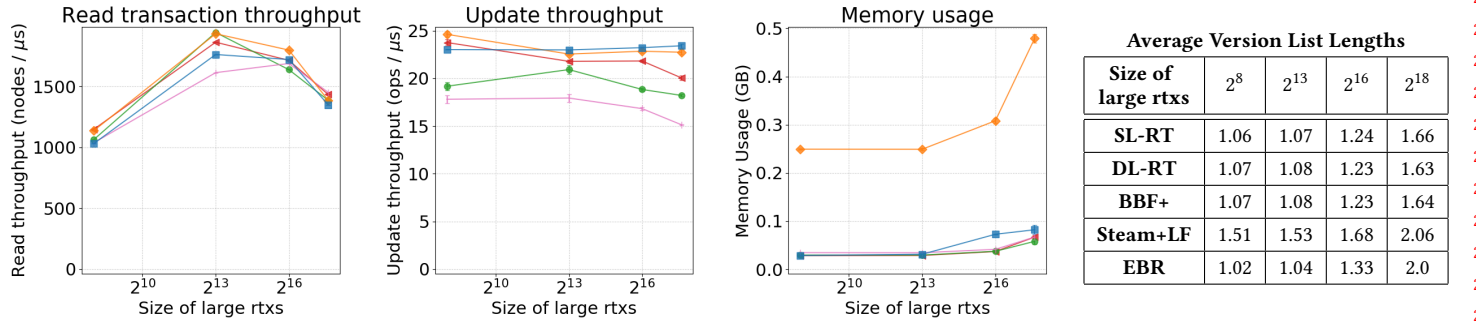

Figure 12. Tree with 100K keys, 40 update threads, 40 small rtx threads, 40 large rtx threads

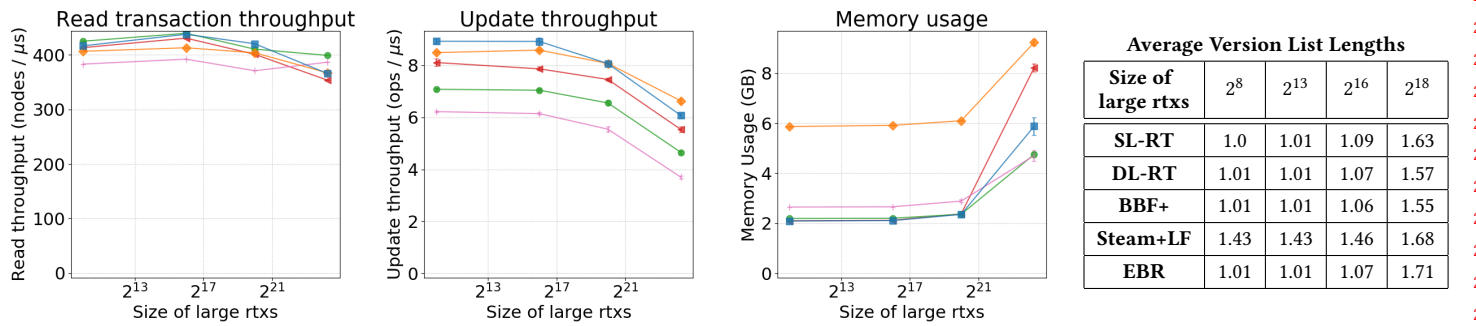

Figure 13. Tree with 10M keys, 40 update threads, 40 small rtx threads, 40 large rtx threads

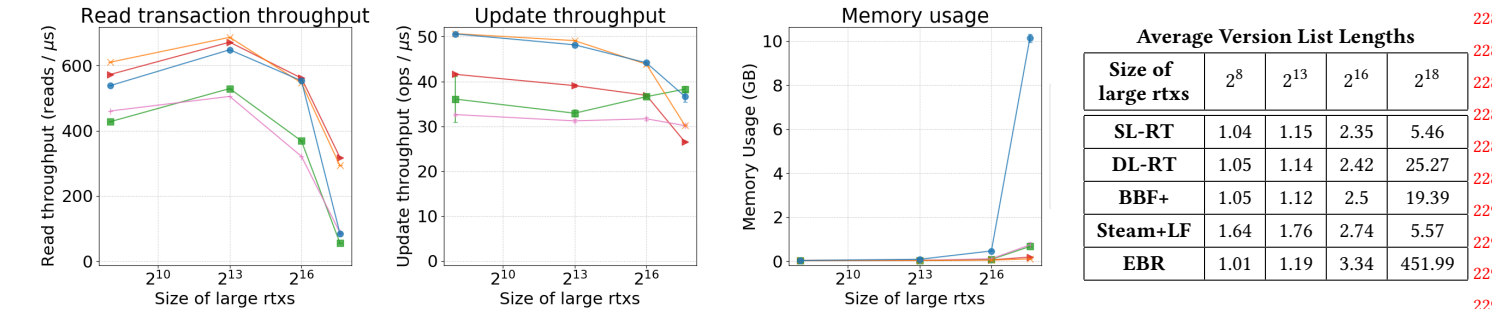

Figure 14. Hash table with 100K keys, 40 update threads, 40 small rtx threads, 40 large rtx threads

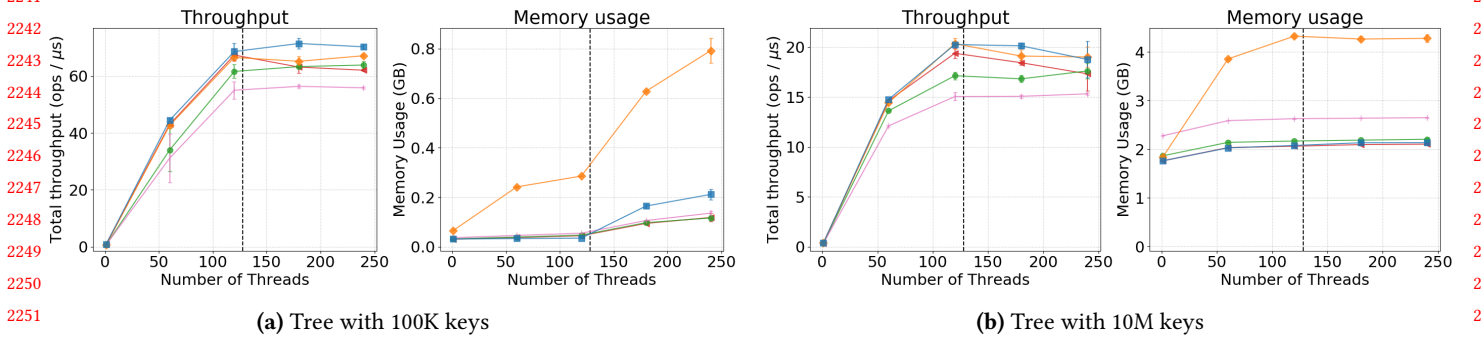

Figure 15. Workload with each thread performing 50% updates and 50% read transactions of size 1024.

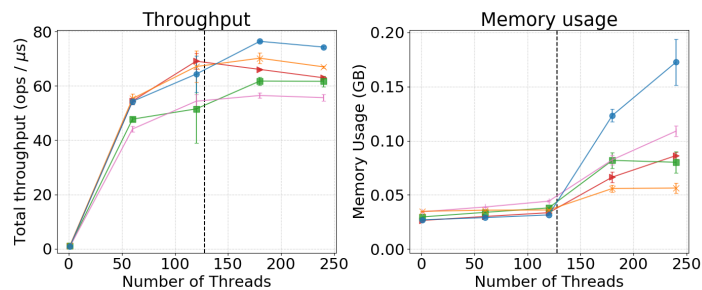

**Figure 16.** Hash table with 100K keys, each thread performs 50% updates and 50% read transactions of size 1024
